# Supplementary material for: InstantIR: Blind Image Restoration with Instant Generative Reference
Source: arXiv:2410.06551 source file (2024-10-09)
Supplement: Supplementary file 1 [file Appendix.tex]

\clearpage
\appendix

\section{More Results}

\begin{table}[h]
\centering
    \begin{tabular}{lcccccc}
    \toprule
    \multirow{2}{*}{\bf Metrics}  &\multicolumn{2}{c}{\bf Synthetic}  &\multicolumn{2}{c}{\bf RealSR}  &\multicolumn{2}{c}{\bf DRealSR}\\
    \cmidrule(lr){2-3}\cmidrule(lr){4-5}\cmidrule(lr){6-7}
        &ControlNet &\methodname   &SUPIR &\methodname   &SUPIR &\methodname\\
    \midrule
    PSNR  &20.46   &18.80 &0  &0  &0  &0\\
    SSIM  &0.5691   &0.5076 &0  &0  &0  &0\\
    LPIPS  &0.4465   &0.3903 &0  &0  &0  &0\\
    CLIPIQA   &0.4618  &0.6111 &0   &0  &0  &0\\
    MANIQA   &0.3237  &0.4303 &0   &0  &0  &0\\
    MUSIQ   &56.44  &66.09 &0   &0  &0  &0\\
    \bottomrule
    \end{tabular}
\label{tab:supir}
\caption{Compare with SUPIR on $1024^2$ real-world data}
\end{table}

\section{Adaptive Restoration Algorithm}

\section{Hyper-Parameters}

\paragraph{LoRA}
